# Supplementary material for: QASem Parsing: Text-to-text Modeling of QA-based Semantics
Source: arXiv:2205.11413 source file (2023-02-14)
Supplement: Supplementary file 1 [file 99_supplementary.tex]

\documentclass[11pt]{article}

% Remove the "review" option to generate the final version.
\usepackage[review]{emnlp2021}
% Standard package includes
\usepackage{times}
\usepackage{latexsym}
% For proper rendering and hyphenation of words containing Latin characters (including in bib files)
\usepackage[T1]{fontenc}
% For Vietnamese characters
% \usepackage[T5]{fontenc}
% See https://www.latex-project.org/help/documentation/encguide.pdf for other character sets

% This assumes your files are encoded as UTF8
\usepackage[utf8]{inputenc}
% This is not strictly necessary, and may be commented out,
% but it will improve the layout of the manuscript,
% and will typically save some space.
\usepackage{microtype}
\usepackage{graphicx}
\usepackage{multirow}
\usepackage{xcolor}
\usepackage{amsmath,amssymb,stackengine}
\usepackage{array}
\usepackage{xcite}
\usepackage{placeins}

\title{Appendices}

\usepackage{biblatex}
\addbibresource{<9_qaalign.bib>}

% set figure & table numbers to reflect appendix_section (e.g. table A.1)

\begin{document}
\maketitle

\appendix
\input{10_appendices}

\end{document}
